# Supplementary material for: Structural Relaxation of Materials with Spin-Orbit Coupling: Analytical Forces in Spin-Current DFT
Source: arXiv:2306.04309 source file (2023-07-20)
Supplement: Supplementary file 1 [file art_of_grad_SM.pdf]

# Analytical Gradients in Spin-Current DFT: Crystal Structure of Solids with Spin-Orbit Coupling

Jacques K. Desmarais\*

*Dipartimento di Chimica, Università di Torino, via Giuria 5, 10125 Torino, Italy*

Alessandro Erba†

*Dipartimento di Chimica, Università di Torino, via Giuria 5, 10125 Torino, Italy*

Jean-Pierre Flament

*Université de Lille, CNRS, UMR 8523 — PhLAM — Physique des Lasers, Atomes et Molécules, 59000 Lille, France*

## I. FINITE DIFFERENCE COEFFICIENTS

TABLE S1: Values of the finite difference coefficients employed in the computations on infinite chains of  $\text{H}_2\text{Po}_2$ .

|    | -2             | -1             | 0  | 1             | 2               |
|----|----------------|----------------|----|---------------|-----------------|
| 2O |                |                | -1 | 1             |                 |
| 2C |                | $-\frac{1}{2}$ | 0  | $\frac{1}{2}$ |                 |
| 4C | $\frac{1}{12}$ | $-\frac{2}{3}$ | 0  | $\frac{2}{3}$ | $-\frac{1}{12}$ |

## II. INPUT DECKS

### A. $\text{H}_2\text{Po}_2$ Polymer

```
H2Po2
POLYMER
1
6.
4
284 0. .0 0.
284 0.3 .0 0.
1 -0.125 .5 -0.5
1 0.425 .5 0.5
OPTGEOM
ENDOPT
END
1 3
0 0 3 1.0 1.0
.1873113696D+02 .3349460434D-01
.2825394365D+01 .2347269535D+00
.6401216923D+00 .8137573262D+00
0 0 1 0.0 1.0
.1612777588D+00 .1000000000D+01
0 2 1 0.0 1.0
```

---

\*Electronic address: [jacqueskontak.desmarais@unito.it](mailto:jacqueskontak.desmarais@unito.it)

†Electronic address: [alessandro.erba@unito.it](mailto:alessandro.erba@unito.it)

```

.1100000000D+01 .1000000000D+01
284 4
STUTLC
0 0 3 2. 1
2.549831 -0.093655
1.856210 0.874894
1.374970 -1.246453
0 0 1 0. 1
0.310166 1.0
0 2 3 4. 1
2.490870 -0.045917
1.843336 0.285716
1.365434 -0.407404
0 2 1 0. 1
0.296807 1.0
99 0
END
TWOCOMPON
SOC
ENDTWO
SHRINK
1000 1000
NOBIPOLA
TOLPSEUD
100
TOLINTEG
100 100 100 1000 1000
TOLDEE
12
MAXCYCLE
300
ENDSCF

```

## B. I<sub>2</sub> Molecule Large-Core

```

I2 large core
MOLECULE
1
2
253 0.000000000000E+00 0.000000000000E+00 -1.410988406779E+00
253 0.000000000000E+00 0.000000000000E+00 1.410988406779E+00
OPTGEOM
MAXCYCLE
1000
ENDOPT
END
253 8
STUTLC
0 0 3 2. 1
5.311170 -0.098005
3.762566 0.297109
1.628957 -0.533922
0 0 1 0. 1
1.163541 1.0
0 0 1 0. 1
0.289886 1.0
0 0 1 0. 1

```

```

0.114132 1.0
0 2 3 5.0 1
5.727873 -0.018074
4.068994 0.062840
1.743004 -0.195622
0 2 1 0. 1
0.378180 1.0
0 2 1 0. 1
0.162712 1.0
0 2 1 0. 1
0.066961 1.0
99 0
END
TWOCOMPON
SOC
ENDTWO
DFT
PBEO
XXLGRID
ENDDFT
FMIXING
70
TOLINTEG
1000000 1000000 1000000 1000000
TOLPSEUD
1000000
NOBIPOLA
TOLDEE
10
MAXCYCLE
1000
END

```

### C. I<sub>2</sub> Molecule Small-Core

```

I2 small core
MOLECULE
1
2
253 0.000000000000E+00 0.000000000000E+00 -1.410988406779E+00
253 0.000000000000E+00 0.000000000000E+00 1.410988406779E+00
OPTGEOM
MAXCYCLE
1000
ENDOPT
END
253 13
STUTSC
0 0 11 2 1
0.55465000E+04 0.15600000E-03
0.83821400E+03 0.98600000E-03
0.18218700E+03 0.27920000E-02
0.31212300E+02 -0.43251000E-01
0.19531400E+02 0.23413400E+00
0.82409900E+01 -0.75094300E+00
0.21945500E+01 0.88296800E+00
0.11091100E+01 0.46206100E+00

```

```

0.37464100E+00 0.22286000E-01
0.17708000E+00 -0.43530000E-02
0.81061000E-01 0.11020000E-02
0 0 11 2 1
0.55465000E+04 -0.73000000E-04
0.83821400E+03 -0.50800000E-03
0.18218700E+03 -0.11580000E-02
0.31212300E+02 0.12193000E-01
0.19531400E+02 -0.87854000E-01
0.82409900E+01 0.33820000E+00
0.21945500E+01 -0.57655000E+00
0.11091100E+01 -0.40929800E+00
0.37464100E+00 0.56745900E+00
0.17708000E+00 0.61248900E+00
0.81061000E-01 0.14323100E+00
0 0 1 0 1
0.37464100E+00 0.10000000E+01
0 0 1 0 1
0.17708000E+00 0.10000000E+01
0 0 1 0 1
0.10010000E+00 0.10000000E+01
0 2 9 6 1
0.18898800E+03 0.58500000E-03
0.21286800E+02 0.36923000E-01
0.10039600E+02 -0.23532400E+00
0.34518000E+01 0.34148300E+00
0.19745600E+01 0.53478800E+00
0.10242000E+01 0.26514100E+00
0.44943700E+00 0.25787000E-01
0.18664800E+00 0.52200000E-03
0.73481000E-01 0.60600000E-03
0 2 9 5 1
0.18898800E+03 -0.25600000E-03
0.21286800E+02 -0.11682000E-01
0.10039600E+02 0.83192000E-01
0.34518000E+01 -0.15697000E+00
0.19745600E+01 -0.22451800E+00
0.10242000E+01 -0.11445100E+00
0.44943700E+00 0.37535600E+00
0.18664800E+00 0.57513600E+00
0.73481000E-01 0.24591700E+00
0 2 1 0 1
0.59810000E+00 0.10000000E+01
0 2 1 0 1
0.96180000E-01 0.10000000E+01
0 3 9 10 1
0.13266200E+03 0.57200000E-03
0.37605400E+02 0.44020000E-02
0.10389100E+02 -0.40922000E-01
0.64901700E+01 0.99661000E-01
0.34545100E+01 0.32266300E+00
0.18441300E+01 0.40034300E+00
0.96247800E+00 0.26830600E+00
0.47285300E+00 0.84847000E-01
0.19320000E+00 0.76320000E-02
0 3 1 0 1
0.47285300E+00 0.10000000E+01
0 3 1 0 1

```

```

0.19320000E+00 0.10000000E+01
0 4 1 0 1
0.40640000E+00 0.10000000E+01
99 0
END
TWOCOMPON
SOC
ENDTWO
DFT
PBEO
XXLGRID
ENDDFT
FMIXING
70
TOLINTEG
1000000 1000000 1000000 1000000 1000000
TOLPSEUD
1000000
NOBIPOLA
TOLDEE
10
MAXCYCLE
1000
END

```

#### D. I2 Molecular Crystal

```

I2 Molecular Crystal
CRYSTAL
0 0 0
64
7.24998540      4.58919224      9.55029852
1
253  3.148405348581E-17  1.593570188084E-01  1.200860777715E-01
SYMMREMO
OPTGEOM
HESSIDEN
CRYDEF
FIXDEF
3
1 3 1.0 1.0
0 4 0.0 0.0
0 5 0.0 0.0
ENDOPT
END
253 9
STUTSC
0 0 3 2. 1
5.311170 -0.098005
3.762566  0.297109
1.628957 -0.533922
0 0 1 0. 1
1.163541 1.0
0 0 1 0. 1
0.289886 1.0
0 0 1 0. 1
0.114132 1.0

```

```

0 2 3 5.0 1
5.727873 -0.018074
4.068994 0.062840
1.743004 -0.195622
0 2 1 0. 1
0.378180 1.0
0 2 1 0. 1
0.162712 1.0
0 3 1 0. 1
0.9      1.0
0 3 1 0. 1
0.3      1.0
99 0
END
TWOCOMPON
SOC
ENDTWO
FMIXING
70
DFT
XXLGRID
PBEO
ENDDFT
TOLPSEUD
8
TOLINTEG
8 8 8 8 20
TOLDEE
8
SHRINK
10 10
MAXCYCLE
1000
END

```

#### E. CsI3 Molecular Crystal

```

CsI3 crystal
CRYSTAL
0 0 0
62
10.96146781      6.92009196      10.17139564
4
255 -1.784426289754E-01  2.500000000000E-01  4.656412834129E-01
253  1.649279722747E-01  2.500000000000E-01  3.671948185783E-01
253  3.740125909191E-01  2.500000000000E-01 -4.428174485748E-01
253 -4.297713518155E-01  2.500000000000E-01 -2.574806489234E-01
SYMMREMO
OPTGEOM
HESSIDEN
CRYDEF
FIXDEF
3
0 2 0.0 0.0
0 4 0.0 0.0
0 5 0.0 0.0
MAXCYCLE

```

200  
ENDOPT  
END

253 14

STUTSC

0 0 5 2 1.0

|              |                 |
|--------------|-----------------|
| 5899.5791533 | 0.000241882693  |
| 898.54238765 | 0.001547404174  |
| 200.37237912 | 0.004283668446  |
| 31.418053840 | -0.039417936275 |
| 15.645987838 | 0.960866919920  |

0 0 2 2 1.0

|              |                |
|--------------|----------------|
| 11.815741857 | 0.759615240910 |
| 6.4614458287 | 0.424955018350 |

0 0 2 0 1.0

|              |                |
|--------------|----------------|
| 2.2210057600 | 0.701255197000 |
| 1.0420511800 | 0.298744803000 |

0 0 1 0 1.0

|              |                |
|--------------|----------------|
| 0.2321271300 | 1.000000000000 |
|--------------|----------------|

0 2 3 6 1.0

|              |                 |
|--------------|-----------------|
| 197.30030547 | 0.000739512269  |
| 20.061411349 | 0.066168450008  |
| 9.7631460485 | -0.285546623480 |

0 2 4 5 1.0

|              |                 |
|--------------|-----------------|
| 12.984316904 | -0.049096186164 |
| 3.6199503008 | 0.389144324820  |
| 2.0232273090 | 0.656108172620  |
| 1.0367490559 | 0.318035516470  |

0 2 1 0 1.0

|              |                |
|--------------|----------------|
| 0.3995601300 | 1.000000000000 |
|--------------|----------------|

0 2 1 0 1.0

|              |                |
|--------------|----------------|
| 0.1221941700 | 1.000000000000 |
|--------------|----------------|

0 3 6 10 1.0

|              |                 |
|--------------|-----------------|
| 119.12671745 | 0.000825960396  |
| 33.404240134 | 0.006837767577  |
| 17.805918203 | -0.010308158997 |
| 4.8990510353 | 0.226704576580  |
| 2.4516753106 | 0.441801139370  |
| 1.1820693432 | 0.367754722250  |

0 3 1 0 1.0

|              |                |
|--------------|----------------|
| 1.0035336200 | 1.000000000000 |
|--------------|----------------|

0 3 1 0 1.0

|              |                |
|--------------|----------------|
| 0.5277932300 | 1.000000000000 |
|--------------|----------------|

0 3 1 0 1.0

|              |                |
|--------------|----------------|
| 0.2009869100 | 1.000000000000 |
|--------------|----------------|

0 4 1 0 1.0

|     |     |
|-----|-----|
| 0.9 | 1.0 |
|-----|-----|

0 4 1 0 1.0

|     |     |
|-----|-----|
| 0.3 | 1.0 |
|-----|-----|

255 8

STUTSC

0 0 3 2 1.0

|                |                 |
|----------------|-----------------|
| 5.877811344300 | 0.128599949830  |
| 4.363153828600 | -0.346325697250 |
| 1.804847515500 | 0.699306370510  |

0 0 1 1 1.0

|                |                |
|----------------|----------------|
| 0.666409630000 | 1.000000000000 |
|----------------|----------------|

0 0 1 0 1.0

|                |                 |
|----------------|-----------------|
| 0.300557260000 | 1.000000000000  |
| 0 0 1 0 1.0    |                 |
| 0.150401350000 | 1.000000000000  |
| 0 2 4 6 1.0    |                 |
| 4.275185615400 | 0.045723074174  |
| 1.965666336000 | -0.250199619760 |
| 0.476891952120 | 0.556608500660  |
| 0.215297495880 | 0.582185534060  |
| 0 2 1 0 1.0    |                 |
| 0.301612360000 | 1.000000000000  |
| 0 2 1 0 1.0    |                 |
| 0.150000770000 | 1.000000000000  |
| 0 3 1 0 1.0    |                 |
| 0.159720620000 | 1.000000000000  |
| 99 0           |                 |
| END            |                 |
| TWOCOMPON      |                 |
| SOC            |                 |
| ENDTWO         |                 |
| F MIXING       |                 |
| 70             |                 |
| DFT            |                 |
| XXLGRID        |                 |
| PBEO           |                 |
| ENDDFT         |                 |
| TOLPSEUD       |                 |
| 8              |                 |
| TOLINTEG       |                 |
| 8 8 8 8 20     |                 |
| TOLDEE         |                 |
| 8              |                 |
| SHRINK         |                 |
| 4 4            |                 |
| MAXCYCLE       |                 |
| 1000           |                 |
| END            |                 |
